# Supplementary material for: Inter-event correlations from avalanches hiding below the detection threshold
Source: arXiv:1610.08324 ancillary file (2016-10-26)
Supplement: Supplementary file 1 [file supplemental_material2.pdf]

# Supplemental Material - Inter-event correlations from avalanches hiding below the detection threshold

Sanja Janićević[1], Lasse Laurson[1,2], Knut Jørgen Måløy[3], Stéphane Santucci[3,4], and Mikko J. Alava[1]
[1]*COMP Centre of Excellence, Department of Applied Physics, Aalto University, P.O. Box 11100, 00076 Aalto, Espoo, Finland*
[2]*Helsinki Institute of Physics, Department of Applied Physics, Aalto University, P.O. Box 11100, 00076 Aalto, Espoo, Finland*
[3]*Department of Physics, University of Oslo, PB 1048 Blindern, NO-0316, Norway and*
[4]*Laboratoire de physique, CNRS UMR 5672, Ecole Normale Supérieure de Lyon, 46 Allée d'Italie, 69364 Lyon Cedex 07, France*

Here, we briefly discuss another experiment giving rise to the same results as the one shown in the main article, and also perform the corresponding analysis of thresholding-induced inter-event correlations within a mean field model. Also more details on the experiment, simulations and data analysis are given.

*Simulations of the crack line model:* We simulate the crack line interface depinning model, Eq. (2) of the main article, with periodic boundary conditions. The parallel dynamics of the interface are defined in discrete time $t$ by setting the local velocity $v_i(t) \equiv h_i(t+1) - h_i(t) = \theta(F_i)$, where $\theta$ is the Heaviside step function. The interface is driven with a constant velocity $\langle V \rangle$ by setting $F_{\text{ext}} = K(\langle V \rangle t - \langle h \rangle)$, with $K$ a parameter analogous to the demagnetizing factor for ferromagnetic domain walls [1], or to the elastic stiffness of the specimen-machine system in a mechanical loading experiment [2]; $K$ controls the cut-off of the avalanche distributions in the quasistatic limit $\langle V \rangle \to 0$, with the cutoff size $S_0$ obeying $S_0 \sim K^{-1/\sigma_K}$, for example. The crackling noise signal of interest is given by $V(t) = 1/L \sum_i v_i(t)$. The simulations are performed in systems of linear size $L = 8192 = 2^{13}$, and by using sufficiently small $K$-values such that the avalanche cutoff $S_0 \sim K^{-1/\sigma_K}$ is large, but the avalanches still fit within the system, and no finite size effects are observed. In practice, $K$ has to be tuned so that the resulting $S_0$ is smaller than $S_{\max} \propto L^{\zeta+1}$, where $\zeta = 0.385 \pm 0.005$ is the roughness exponent of the long-range elastic string [3]. An example of the crackling noise signal $V(t) = 1/L \sum_i v_i(t)$ obtained from the model for $\langle V \rangle = 0.01$ and $K = 0.0006$ is shown in the bottom right inset of Fig. 1 of the main article.

*Planar crack front propagation experiments:* We have studied the intermittent crack front propagation along the heterogeneous weak plane of a transparent poly(methyl methacrylate) (PMMA) block. This block was made of two sintered rough (sand-blasted) Plexiglas plates, annealed together at 205 °C under several bars of normal pressure. A normal displacement at a constant velocity was imposed to the bottom plate of dimensions 32 × 14 × 1 cm, while the upper one [of dimensions 34 × 12 × 0.4 cm] was fixed, leading to a quasi-mode I growth of the crack. Using a high-resolution fast camera mounted on a microscope, we directly observed the interfacial crack front propagation. We recorded typically 10 000 images of 1024 × 512 pixels at a rate of 1000 frames per second in a small central region of the sample (to avoid boundary effects). In the main article, we consider an experiment with the pixel size $r = 1.7$ $\mu$m, smaller than the typical disorder size due to the sand-blasting procedure, and the average crack front velocity $\langle V \rangle = 10.2$ $\mu$m/s; other choices of $\langle V \rangle$ and $r$, yielding the same results, are discussed later in this Supplemental Material.

The spatially random toughness along the weak interface leads to intermittent avalanche dynamics of the crack front. We consider here the global spatially averaged velocity of the crack front $V(t)$ (see the top right inset of Fig. 1 of the main article for an example), computed at the scale of 217 $\mu$m, larger than the correlation length of the order of 100 $\mu$m of the local front velocities along the crack front. The local front velocities $v(x,y)$ were obtained from measurements of the local waiting times $wt(x,y)$ elapsed while the crack front was located at a given position $(x,y)$, and defining $v(x,y) = r/wt(x,y)$ [4, 5]. Thus, we have 8 crackling noise signals, with the total number of avalanches detected depending on $V_{\text{th}}$ as shown in the bottom right inset of Fig. 2a of the main article, or in the bottom right inset of Fig. S2 for the other experiment with other $\langle V \rangle$ and $r$ values.

*Scaling of $\langle S(T) \rangle$ with $T$ for different $V_{th}$:* In Fig. 2 of the main text, the scaling of $\langle S(T) \rangle$ with $T$ is analyzed for different $V_{\text{th}}$, and an effective $V_{\text{th}}$-dependent $\gamma$-exponent is found. The fitting range to extract the effective $\gamma$-value is chosen such that in each case (i.e., for each $V_{\text{th}}$-value), the fit is limited to the intermediate-$T$ range, in order to avoid spurious effects from very small avalanches, and those due to the large avalanche cutoff, as shown by the solid lines in Fig. S1, where only a subset of the data shown in Fig. 2 of the main text is shown magnified for clarity. We emphasize that the resulting $\gamma$ for any finite $V_{\text{th}}$ is an effective exponent, and our results illustrate that it can be dangerous to make far-reaching conclusions based on exponent values from experiments where thresholding is used, without properly examining the dependence of the results on the threshold level $V_{\text{th}}$.

A possible explanation for the decreasing value of the

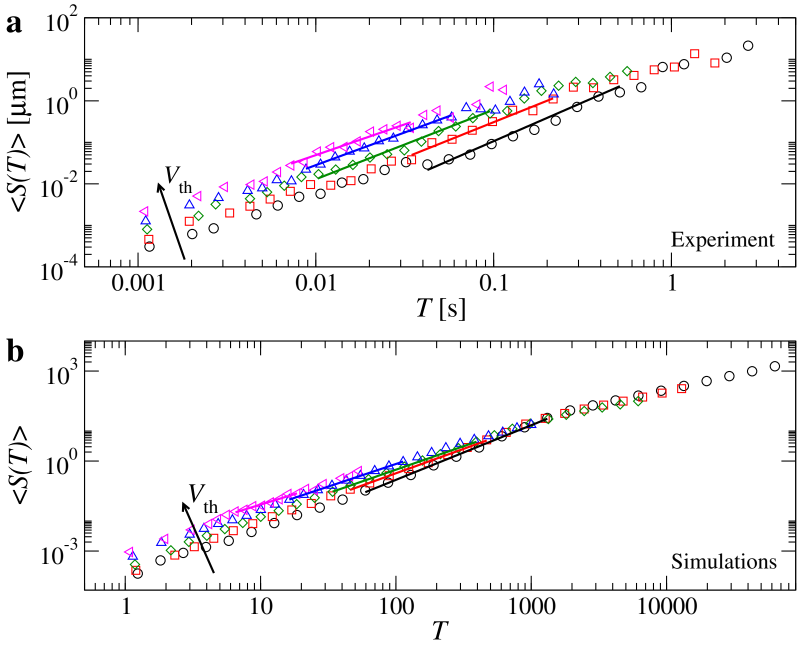


FIG. S1. Magnified version of a subset of the data shown in Fig. 2 of the main text, i.e., the scaling of $\langle S(T)\rangle$ with $T$ for different threshold levels $V_{\rm th}$, showing also power law fits to the data (solid lines). **a** shows data from the experiment discussed in the main text (and shown in Fig. 2a) while **b** displays numerical data corresponding to that shown in Fig. 2b of the main text. In each case, the fitting range to extract the effective $V_{\rm th}$-dependent $\gamma$-value (shown in the top left insets of Fig. 2 of the main text), indicated by the solid lines, is chosen from the intermediate-$T$ range, in order to avoid spurious effects from very small avalanches, and those due to the large avalanche cutoff. In practice this leads to considering roughly the same, although increasingly narrow range in $S$ with increasing $V_{\rm th}$.

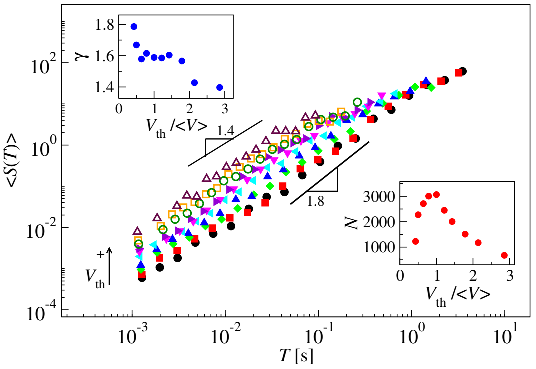


FIG. S2. Scaling of the average avalanche size $\langle S(T)\rangle$ with the avalanche duration $T$ for a crack propagation experiment with $\langle V\rangle = 24.5$ μm/s, pixel size $r = 3.5$ $\mu$m, and observation scale of 224 $\mu$m. The top left inset shows the evolution of the effective value of the $\gamma$-exponent with the threshold level $V_{\rm th}$; the fitting range used evolves with $V_{\rm th}$ roughly as indicated by the two slopes (solid black lines in the main panel). The bottom right inset shows the $V_{\rm th}$ dependence of the number of avalanches recorded. The results are essentially the same as for the other experiment with a different $\langle V\rangle$ discussed in the main article.

effective $\gamma$-exponent with $V_{\rm th}$ could be that it is due to the cutoff mechanism limiting the growth of avalanches due to the driving mechanism: Indeed, since the cutoff due to the constant velocity drive limits the $V(t)$-values, avalanches of increasing duration should have a tendency to be smaller in relative terms (or, increase in size more slowly with $T$) when they are extracted using a higher threshold level $V_{\rm th}$. This effect is visible also as the smaller slope of the longest low-threshold avalanches in Fig. 2 of the main text (data points towards the right side of the panels). For high thresholds, this lower slope shifts towards shorter avalanches, thus resulting in a smaller effective value of $\gamma$.

*Analysis of the probability distributions:* To extract estimates of the critical exponents $\tau_T$ and $\tau_{T_{\rm W}}$ (as well as $\tau_S$ and $\tau_{S'}$, see below) characterizing the probability distributions $P(T)$ and $P(T_{\rm W})$, respectively, we fit the distributions with functions of the form of (for the avalanche durations $T$)

$$P(T) = AT^{-\tau_T}\exp(B\sqrt{T} - CT^{\alpha}), \tag{S1}$$

where $\tau_T$, $A$, $B$, $C$ and $\alpha$ are fitting parameters. An analogous form is used for the waiting times $T_{\rm W}$ (as well as for $S$ and $S'$), obtained by making the substitution $T \to T_{\rm W}$. This form allows for the presence of a small "bump" in the cutoff, something we cannot exclude *a priori*, and has been predicted to describe avalanche size

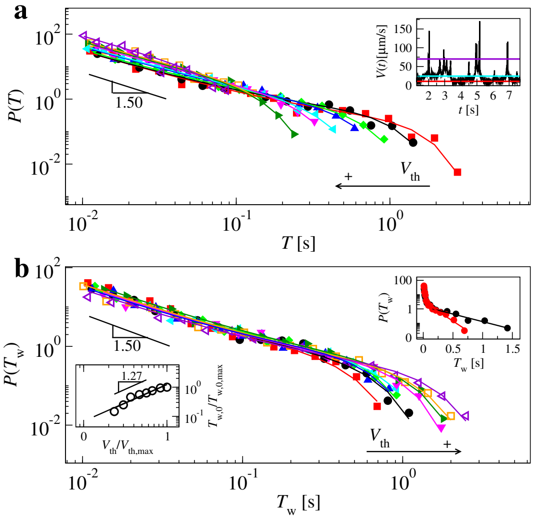


FIG. S3. Avalanche duration and waiting time distributions for a crack propagation experiment with $\langle V \rangle = 24.5$ $\mu$m/s, pixel size $r = 3.5$ $\mu$m, and observation scale of 224 $\mu$m (i.e. the same experiment as shown in Supplemental Material Figure S1). **a**, main panel, shows the duration distributions $P(T)$ for a wide range of threshold levels $V_{\mathrm{th}}$; the bottom and top horizontal lines in the inset correspond to the minimum and maximum $V_{\mathrm{th}}$ values considered, while the middle one indicates the mean value of the signal (i.e. $\langle V \rangle$). **b**, main panel, shows the corresponding waiting time distributions $P(T_{\mathrm{W}})$; the top right inset shows the $P(T_{\mathrm{W}})$'s for the two lowest $V_{\mathrm{th}}$-values on a semilog axis scale, showing that they are well-described by exponentials. Bottom left inset shows the scaling of the cut-off waiting time with $V_{\mathrm{th}}$, consistent with $\delta \approx 1.3$. The results are essentially the same as for the other experiment with a different $\langle V \rangle$ discussed in the main article.

distributions close to the depinning transition of non-mean field systems by functional renormalization group calculations [6]. Eq. (S1) allows us to obtain estimates of the values of $\tau_T$ and $\tau_{T_{\mathrm{W}}}$ unbiased by the shape of the cutoff, resulting in $\tau_{T_{\mathrm{W}}} \approx \tau_T = 1.53 \pm 0.05$ for both experiments and simulations; notice that this $\tau_T$ value is in agreement with previous results via the scaling relation $\tau_T = \gamma(\tau_S - 1) + 1$ [8, 9]. The solid lines shown in Figs. 3 and 4 of the main article, as well as in Figs. S3 and S6, show the best fits of Eq. (S1) to the data.

*Experiment with $r$ = 3.5 $\mu$m and $\langle V \rangle$ = 24.5 $\mu$m/s:* Fig. S2 shows the scaling of the average avalanche size $\langle S(T) \rangle$ with the avalanche duration $T$ for a crack propagation experiment with $\langle V \rangle = 24.5$ $\mu$m/s, pixel size $r = 3.5$ $\mu$m, and observation scale of 224 $\mu$m; the results are essentially the same as those presented in Fig. 2a of the main article for another experiment with $r = 1.7$ $\mu$m and $\langle V \rangle = 10.2$ $\mu$m/s. Distributions of avalanche durations $T$ and waiting times $T_{\mathrm{w}}$ for the same experiment are shown in Fig. S3. Also these results are in agreement with those presented in Figs. 3a and b of the main article, demonstrating that our results are not sensitive to the details

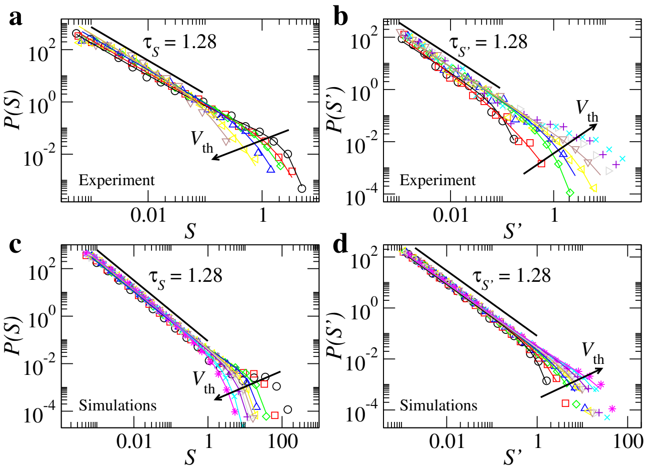


FIG. S4. Distributions $P(S)$ and $P(S')$ of the areas $S$ (i.e., the avalanche sizes) and $S'$ of the excursions of $V(t)$ above and below $V_{\mathrm{th}}$, respectively. **a** and **b** show the experimental $P(S)$ and $P(S')$ for different threshold levels $V_{\mathrm{th}}$, respectively, while **c** and **d** display the corresponding distributions from the simulations. The same datasets as shown in Fig. 3 of the main article are considered here. The arrows indicate the direction in which $V_{\mathrm{th}}$ increases. Thick black solid lines serve as guides to the eye, and correspond to the typical value of 1.28 of the exponents $\tau_S$ and $\tau_{S'}$, obtained by fitting a function of the form of Eq. (S1) to the data; the fits are shown as thin solid lines.

(driving velocity, etc.) of the experiment.

*"Statistical symmetry" of excursions of $V(t)$ above and below $V_{th}$:* Since the argument that the thresholding-induced power-law scaling of waiting times $T_{\mathrm{W}}$ is characterized by the same exponent as the one describing the avalanche duration distributions $P(T)$ hinges on the concept of "statistical symmetry" of excursions of $V(t)$ above and below a finite threshold $V_{\mathrm{th}}$, we provide here additional evidence supporting it. In particular, we consider the distributions of the avalanche sizes $S = \int_0^T dt[V(t) - V_{\mathrm{th}}]$ (i.e., the areas of the excursions of $V(t)$ above $V_{\mathrm{th}}$, see also Fig. 1 of the main text), and the corresponding areas $S'$ of the excursions of duration $T_{\mathrm{W}}$ *below* $V_{\mathrm{th}}$, i.e., $S' = \int_0^{T_{\mathrm{W}}} dt[V_{\mathrm{th}} - V(t)]$. Fig. S4 shows that for experimental and numerical data, both the $P(s)$ and $P(s')$ distributions exhibit a clear power law scaling regime with an exponent $\tau_S \approx \tau_{S'} \approx 1.28$. This value is close to the $\tau_S$-value $\tau_S \approx 1.25$ found before in the limit of $V_{\mathrm{th}} \to 0$ in numerical studies of the crack line model [7]. Thus, up to their $V_{\mathrm{th}}$-controlled cutoff scales (exhibiting again the opposite dependence on $V_{\mathrm{th}}$ for $P(S)$ and $P(S')$, see Fig. S4), the excursions of $V(t)$ above and below $V_{\mathrm{th}}$ are indeed found to be statistically symmetric also in this sense.

*On the $V_{th} \to 0$ limit of the waiting time distributions:* Here, we have found that in the limit of zero threshold and driving velocity, the waiting time distributions be-

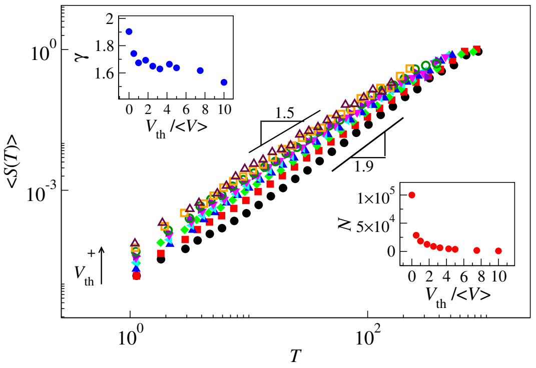


FIG. S5. Scaling of the average avalanche size $\langle S(T)\rangle$ with the avalanche duration $T$ for the mean field model discussed in this Supplemental Material in the quasistatic limit $\langle V\rangle \to 0$. The top left inset shows the evolution of the effective value of the $\gamma$-exponent with the threshold level $V_{\rm th}$; it evolves from a value close to the theoretical result $\gamma = 2$ towards 1.5 as $V_{\rm th}$ is increased. This behavior is qualitatively similar to that observed for the crack propagation experiments and simulations of the crack line model (see Fig. 2 of the main article, and Supplemental Material Figure S2). The bottom right inset shows the $V_{\rm th}$ dependence of the number of avalanches recorded, which here has (due to the $\langle V\rangle \to 0$ considered) a different shape as compared to those for the finite rate crack propagation experiments and simulations.

come Poissonian (Fig. 4 of the main article), and that $P(T_{\rm W})$s with a power law form are observed only for a finite $V_{\rm th}$. The former is in agreement with previous results for driven elastic interfaces in random media [10], which in general correspond to long-range correlated disorder acting on the center of mass of the interface: for such systems, both the sizes and the time occurrences of the events are typically found to be almost uncorrelated variables [10]. In contrast, for point particles driven through short-range correlated disorder with a constant velocity drive, an equivalence of $P(T_{\rm W})$ and the avalanche size distribution $P(S)$ has been established [11]. However, even for such a system, $P(T_{\rm W})$ [as well as $P(S)$] does not assume a power law form, as the relevant exponent values are found to be $\tau_{T_{\rm W}} = \tau_S = 0$ [11].

*Mean field interface depinning model:* The mean field limit of the class of interface depinning models to which also the crack line model discussed in the main article belongs is obtained by replacing the elastic interaction term by an infinite range elastic interaction, such that Eq. (2) of the main article becomes

$$F_i = \langle h\rangle - h_i + \eta(x_i, h_i) + F_{\rm ext}. \qquad \text{(S2)}$$

The resulting model is known to belong to the mean field universality class characterized by exponents $\tau_S = 3/2$, $\tau_T = 2$ and $\gamma = 2$ in the $\langle V\rangle \to 0$ limit (see e.g. ref. 4 of the main text, or ref. [8], and references therein). Thus, within our scaling description of the thresholding-induced waiting times presented in the main article, one

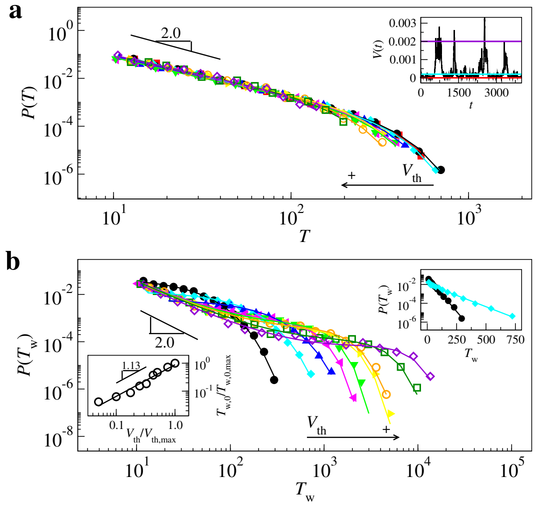


FIG. S6. **a** Avalanche duration distributions $P(T)$ for different threshold levels $V_{\rm th}$ from the mean field model discussed in this Supplemental Material. The scaling exponent $\tau_{\rm T}$ is close to the theoretically expected value $\tau_T = 2$. The inset indicates the minimum and maximum threshold levels used, as well as the mean value of the signal (the middle horizontal line). **b** shows the corresponding waiting time distributions $P(T_{\rm W})$. While for small $V_{\rm th}$ the $P(T_{\rm W})$'s are exponential (top right inset), for large enough $V_{\rm th}$, they develop a power-law part with an exponent $\tau_{T_{\rm W}} \approx \tau_T \approx 2$. The bottom left inset shows the dependence of the cut-off waiting time $T_{\rm W,0}$ on the threshold level $V_{\rm th}$, exhibiting close to linear scaling. These results show that also the mean field model obeys our scaling picture of the thresholding-induced power-law waiting times.

would expect the waiting times to be power-law distributed with an exponent $\tau_{T_{\rm W}} = \tau_T = 2$ and the cut-off scale to be linearly dependent on the threshold level, $T_{\rm W,0} \propto V_{\rm th}$, in the limit $\langle V\rangle \to 0$. Supplemental Material Figures S5 and S6 show results from simulations of the mean field model with the $\langle V\rangle \to 0$ limit reached by triggering avalanches by increasing $F_{\rm ext}$ just enough to make exactly one interface element unstable (that is, $F_i > 0$ for some $i$) whenever the previous avalanche has ended, and by decreasing $F_{\rm ext}$ during avalanches at a rate proportional to the instantaneous avalanche velocity, $F_{\rm ext} = -KV(t)$. These simulations show that indeed our scaling description works also for the mean field model, in that the waiting time distributions develop a power law part with an exponent close to $\tau_{T_{\rm W}} = 2$ for high enough threshold values $V_{\rm th}$ (which agrees with the scaling exponent close to $\tau_T = 2$ of the avalanche duration distributions for *low* thresholds). The slow evolution of the waiting time distributions with the threshold towards this power law scaling may be related to effects discussed in ref. 32 of the main text. Thus, this agreement of the mean field model with our scaling picture further demonstrates its general applicability to systems exhibiting crackling noise.

[1] G. Durin and S. Zapperi, Universality and size effects in the Barkhausen noise, J. Appl. Phys. **87**, 7031-7033 (2000).

[2] F. Csikor, C. Motz, D. Weygand, M. Zaiser, and S. Zapperi, Dislocation Avalanches, Strain Bursts, and the Problem of Plastic Forming at the Micrometer Scale, Science **318** 251-254 (2007).

[3] O. Duemmer and W. Krauth, Depinning exponents of the driven long-range elastic string, J. Stat. Mech. P01019 (2007).

[4] K. J. Måløy, S. Santucci, J. Schmittbuhl, and R. Toussaint, Local Waiting Time Fluctuations along a Randomly Pinned Crack Front, Phys. Rev. Lett. **96**, 045501 (2006).

[5] K. T. Tallakstad, R. Toussaint, S. Santucci, J. Schmittbuhl, and K. J. Måløy, Local dynamics of a randomly pinned crack front during creep and forced propagation: An experimental study, Phys. Rev. E **83**, 046108 (2011).

[6] A. Rosso, P. Le Doussal, and K. J. Wiese, Avalanche-size distribution at the depinning transition: A numerical test of the theory, Phys. Rev. B **80**, 144204 (2009).

[7] L. Laurson, S. Santucci, and S. Zapperi, Avalanches and clusters in planar crack front propagation, Phys. Rev. E **81**, 046116 (2010).

[8] L. Laurson, X. Illa, S. Santucci, K. T. Tallakstad, K. J. Måløy, and M. J. Alava, Evolution of the average avalanche shape with the universality class, Nat. Commun. **4**, 2927 (2013).

[9] D. Bonamy, S. Santucci, and L. Ponson, Crackling Dynamics in Material Failure as the Signature of a Self-Organized Dynamic Phase Transition, Phys. Rev. Lett. **101**, 045501 (2008).

[10] E. A. Jagla, F. P. Landes, and A. Rosso, Viscoelastic Effects in Avalanche Dynamics: A Key to Earthquake Statistics, Phys. Rev. Lett. **112**, 174301 (2014).

[11] P. Le Doussal and K. J. Wiese, Driven particle in a random landscape: Disorder correlator, avalanche distribution, and extreme value statistics of records, Phys. Rev. E **79** 051105 (2009).
